# Supplementary material for: Sol-gel synthesized double perovskite Gd$_{2}$FeCrO$_{6}$ nanoparticles: Structural, magnetic and optical properties
Source: arXiv:2111.04021 source file (2021-11-07)
Supplement: Supplementary file 1 [file appendix1.tex]

\section{Supplementary Material} \label{sec:appendix}
    Here the ESI will be included.
